# Supplementary material for: MUIT: A Middleware for Adaptive Mobile Web-based User Interfaces in WS-BPEL
Source: arXiv:1602.09125 source file (2016-02-19)
Supplement: Supplementary file 1 [file appendix.tex]

\subsection{MUIT UI Syntax}
